# Supplementary material for: Quantum teleportation over thermal microwave network
Source: arXiv:2508.14691 ancillary file (2025-10-14)
Supplement: Supplementary file 1 [file ThermalTeleportationPaper_SupplementaryMaterial.pdf]

# Supplementary Material for
# "Quantum teleportation over thermal microwave network"

W. K. Yam,[1,2,*] S. Gandorfer,[1,2] F. Fesquet,[1,2] M. Handschuh,[1,2]
K. E. Honasoge,[1,2] A. Marx,[1] R. Gross,[1,2,3] and K. G. Fedorov[1,2,3,†]

[1] *Walther-Meißner-Institut, Bayerische Akademie der Wissenschaften, 85748 Garching, Germany*
[2] *School of Natural Sciences, Technical University of Munich, 85748 Garching, Germany*
[3] *Munich Center for Quantum Science and Technology (MCQST), 80799 Munich, Germany*

[*] WunKwan.Yam@wmi.badw.de
[†] Kirill.Fedorov@wmi.badw.de

# I. EXPERIMENTAL IMPLEMENTATION

## A. Devices and experimental setup

The cryogenic system used in our experiment consists of two dilution refrigerators (Alice and Bob) separated by 6.6 m and connected with a cryogenic link via a cold network node (Eve) [1], as illustrated in Supplementary Fig.1. The mixing chamber (MC) shields of Alice and Bob are connected by a copper tube that runs through the cryogenic link. This allows us to directly connect the microwave devices in Alice and Bob using 6-meter-long superconducting niobium-titanium (NbTi) coaxial cables, which have losses of around $1\,\mathrm{dB\,km^{-1}}$. At their MC stages, the Alice and Bob fridges reach temperatures of 43 mK and 29 mK, respectively. In order to simulate a hot communication channel, we clamp a heater and thermometer onto the NbTi cables at the center of the cryogenic link. Using this PID-controllable heater, we can increase the local temperature, $T_{\mathrm{cen}}$, at the center of the cryogenic link from its 170 mK base temperature up to 4 K.

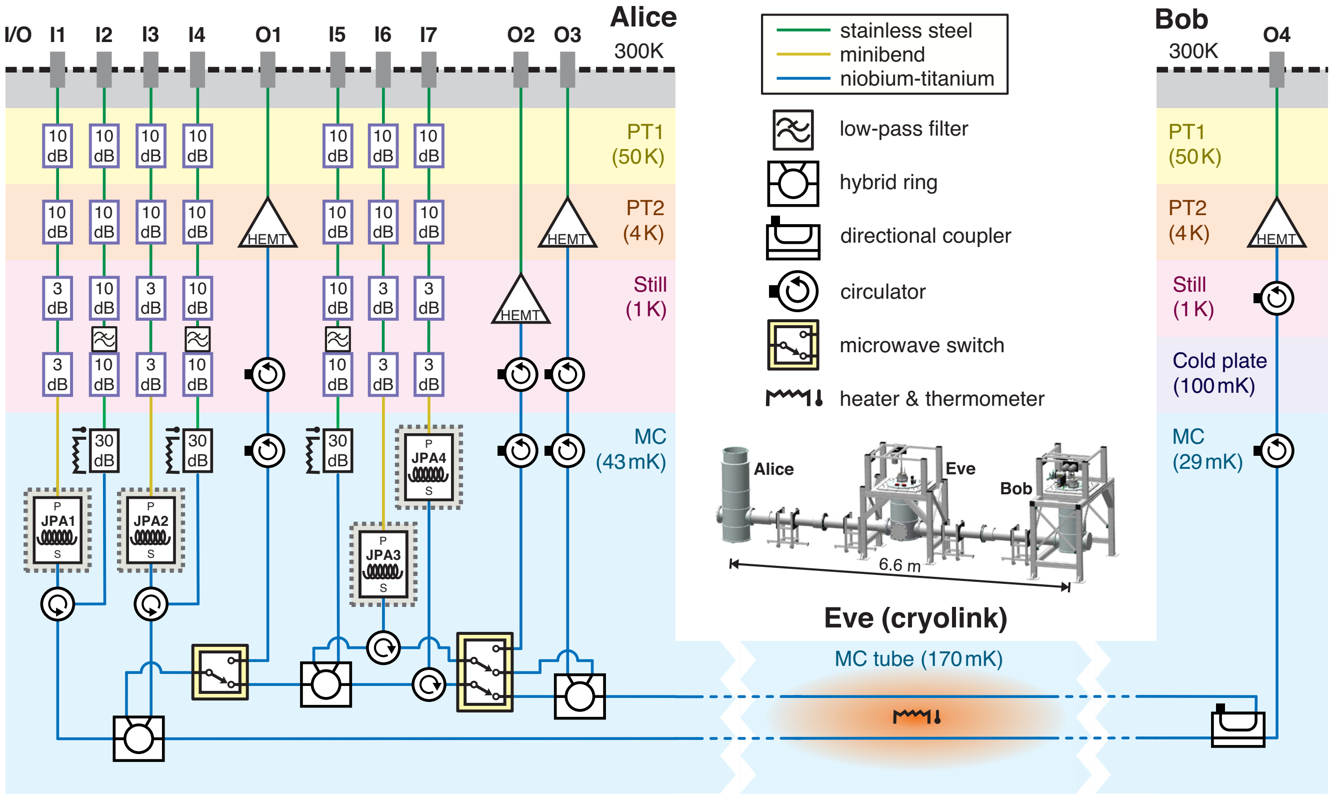


Supplementary Figure 1. Schematic of experiment setup for quantum teleportation over the cryogenic link.

We generate our quantum states in Alice and let them propagate towards Bob, as shown by the schematic in Supplementary Fig. 1. In order to attain a low thermal population in our propagating photonic mode, we place 30 dB attenuators at the superconducting input lines, which match the photonic mode temperature with the Alice MC background temperature. Additionally, PID-controllable heaters are attached to these 30 dB attenuators, which allow us to calibrate the photon number of our quantum states using Planck spectroscopy [2, 3]. Attached to the Alice MC stage are four flux-driven Josephson parametric amplifiers (JPAs) fabricated of aluminum on silicon substrates [4]. Each JPA consists of a superconducting $\lambda/4$ resonator terminated by a dc-SQUID, which enables flux-tuning of the JPA resonance frequency $\omega_0$. The JPAs can be used to perform a squeezing operation by introducing a strong coherent pump tone with frequency $\omega_{\mathrm{p}} = 2\omega_0$ [5, 6]. For our experiment, we tune all four JPAs to the signal frequency $\omega_0/2\pi = 5.35\,\mathrm{GHz}$ by applying external magnetic fields generated by superconducting coils. We enclose each JPA, along with its corresponding superconducting coil, inside a superconducting aluminum box in order to avoid crosstalk between the magnetic fields applied to each JPA. The JPAs in our setup are measured in reflection, where circulators separate the input and output signals. For state tomography, the output quantum signals are amplified, downconverted, and detected by a field-programmable gate array (FPGA). We use the statistical moments up to second order to reconstruct our quantum states in the Gaussian approximation [7], and then use moments up to fourth order to check for Gaussianity.

### B. Implementation of microwave quantum teleportation

Two-mode squeezing (TMS) is an important continuous-variable entanglement resource for various protocols. One method to experimentally generate TMS states is by employing two "entanglement JPAs" (JPA1 and JPA2 in Supplementary Fig. 1) tuned to the same signal frequency. Each JPA is used to generate a single-mode squeezed state with the same squeezing level $S$, but squeezed along orthogonal field quadratures. These two single-mode squeezed states are then superimposed via a hybrid ring, which functions as a balanced beam splitter. The two outgoing modes will appear locally as thermal states but contain nonlocal quantum correlations at the signal frequency $\omega_0$, embodying a TMS state [8]. In our experiment, we generate such TMS states and distribute the two modes between Alice and Bob via the cryogenic link. We then use the shared entanglement to perform quantum teleportation across our 6.6 m-separated dilution refrigerators and study how the quantum properties of propagating microwave states are affected by increasing the cryogenic link center temperature $T_{\mathrm{cen}}$.

We implement an analog (or measurement-device-free [9]) quantum teleportation of coherent states [10], as illustrated in Supplementary Fig. 1. First, we distribute a TMS state with squeezing level $S_{\mathrm{TMS}}$ between Alice and Bob as our entanglement resource. Then, we perform a Bell-type measurement, using a Josephson interferometer [11], on Alice's input coherent state and her part of the TMS state. The Josephson interferometer is composed of two "measurement JPAs" (JPA3 and JPA4 in Supplementary Fig. 1) placed in an interferometer configuration, which makes projective measurements on two selected quadratures when the JPAs are operated in the limit of high degenerate gain $G \gg 1$ [12]. Here, we choose to measure orthogonal quadratures and feed forward the analog measurement result to Bob via the cryogenic link. Finally, we perform a local operation on Bob's part of the TMS state, conditioned upon the feedforward signal. This is accomplished by a directional coupler with coupling $\eta$, which functions as an imbalanced beamsplitter. The directional coupler implements a displacement operation on Bob's part of the TMS state by injecting a small portion of the feedforward signal [13]. In order to perform the correct amount of displacement, we need to match the amplification of the Josephson interferometer with the coupling of the directional coupler, requiring $G = 4\eta$ in the ideal case. For our experiment, we use a directional coupler with $\eta = 15\,\mathrm{dB}$ and hence operate the measurement JPAs around $G = 21\,\mathrm{dB}$. After the output of the directional coupler, we should ideally obtain a coherent state with displacement matching that of Alice's input state and variance at the vacuum level. This reconstructs the input state at Bob, thereby completing quantum teleportation.

Quantum teleportation can be characterized by the fidelity, $F$, between Alice's input and Bob's output states [7, 14]. Without quantum entanglement, arbitrary coherent states can be teleported with average fidelity up to $F_{\mathrm{cl}} = 1/2$, which defines the asymptotic classical threshold [15]. Furthermore, due to the no-cloning theorem, reconstruction of arbitrary coherent states can be considered unique only if its average fidelity exceeds the asymptotic no-cloning threshold of $F_{\mathrm{nc}} = 2/3$ [16]. For the analog quantum teleportation protocol, achieving fidelities of $F > F_{\mathrm{nc}}$ requires a TMS entanglement resource with squeezing below half the vacuum level, $S_{\mathrm{TMS}} < 10\log_{10} 2 \approx 3\,\mathrm{dB}$.

## II. HEATING PROCEDURE AND CALIBRATION

We use the cryolink to mimic a noisy thermal communication channel [1] by heating its center temperature up to $T_{\mathrm{cen}} = 4\,\mathrm{K}$. This is accomplished by using a PID-controlled heater clamped to the NbTi cables at the center of the cryolink. However, this constant local heating also affects the MC temperatures of the Alice and Bob cryostats, as shown in Supplementary Fig. 2(a), due to a finite thermal coupling to the center heater. This coupling results in the increased MC temperatures, which become unsustainable in the steady-state regime for $T_{\mathrm{cen}} \gtrsim 1\,\mathrm{K}$ due to the dilution refrigeration cycle breaking down. Ultimately, we are limited by the cooling power of Alice, which is smaller than that of Bob in the millikelvin temperature range. In order to comply with this limitation, we adopt two heating methods: (i) the steady-state method for $T_{\mathrm{cen}} \leq 1\,\mathrm{K}$ and (ii) the pulsed method for $T_{\mathrm{cen}} > 1\,\mathrm{K}$. The steady-state heating method is displayed by open square markers in Supplementary Fig. 2, where we stabilize $T_{\mathrm{cen}}$ for at least two hours before starting actual microwave protocols. This waiting time ensures that all components of our cryogenic system are well-thermalized. The pulsed method, corresponding to filled circle markers in Supplementary Fig. 2, is less optimal but allows us to access the high temperature range. Here, we stabilize $T_{\mathrm{cen}}$ to a target temperature for around one minute, measuring during this period, and then immediately turn off the heater before the Alice MC temperature rises above the cryostat breakdown threshold. Average temperatures of the Alice MC, Bob MC, and MC tube during the steady-state and pulsed heating methods are shown in Supplementary Fig. 2(a). Although we use two different methods to heat the cryolink center, we observe that the physical implications for propagating microwave states are very similar.

Supplementary Figure 2(b,c) shows the measured negativity and purity values of the TMS states distributed between Alice and Bob at various $T_{\mathrm{cen}}$. In order to compare measurement results of the steady-state and pulsed heating methods, we calibrate the $T_{\mathrm{cen}}$ values using the Alice MC temperature as a common baseline. This approach is

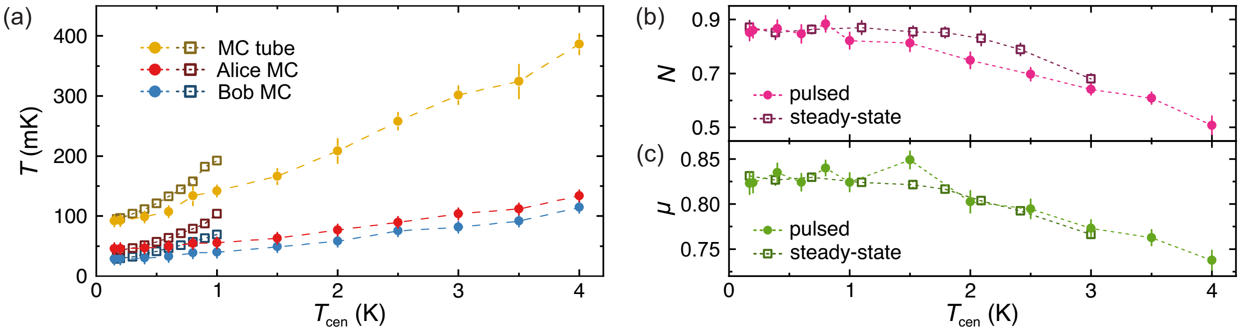


Supplementary Figure 2. Calibration of cryolink heating up to 4 K. (a) Average temperatures $T$ of various MC sections as a function of the cryolink center temperature $T_{\text{cen}}$. Open square and filled circle markers represent measurements of the steady-state and pulsed heating methods, respectively. (b) Negativity $N$ and (c) purity $\mu$ of the TMS states as a function of $T_{\text{cen}}$. Error bars denote standard error of the experimental data and are smaller than the symbol size when not shown.

motivated by our theoretical model (see Section IV of the Supplemental Material), which predicts that the admixed noise is dominated by losses in the Alice setup. In particular, coupling to the ambient thermal bath is strongest at the 30 dB heatable attenuators in Alice, which also absorb back-scattered thermal radiation from the noisy cryolink channel and re-emits weak thermal states as input states for the entanglement JPAs. The propagation losses in the quantum link and the Bob setup itself are estimated to be around 0.01 dB and 0.3 dB, respectively, which are much lower than the aforementioned 30 dB. Since the fluctuation-dissipation theorem states that the noise power density of a system corresponds to its dissipation spectrum [17], we determine that the microwave photonic temperature in an experimentally relevant bandwidth is mainly defined by the Alice MC temperature. Thus, we can calibrate the temperatures obtained in the pulsed heating method in relation to temperatures from the steady-state method through the Alice MC temperature. As an example, $T_{\text{cen}} = 1\,\text{K}$ in the steady-state regime causes the Alice MC temperature to reach 104 mK, which is equivalent to the effect of $T_{\text{cen}} = 3.0\,\text{K}$ in the pulsed method. This conversion procedure is verified by the fact that our measurements result in comparable values of $N$ and $\mu$ for these two heating methods. We see in Fig. 2(b) that $N$ decreases from $0.851 \pm 0.024$ to $0.508 \pm 0.027$ as $T_{\text{cen}}$ rises from 0.17 K to 4 K. This decrease in entanglement can be attributed to additional thermal noise, as shown in Fig. 2(c), where $\mu$ decreases from $0.823 \pm 0.010$ to $0.737 \pm 0.009$. Importantly, $N$ remains above zero, demonstrating that quantum entanglement survives even when passing through a hot quantum link.

## III. QUANTUM COMMUNICATION THROUGH A THERMAL CHANNEL

Quantum communication of photons through a thermal channel is possible, despite large ambient thermal noise, when the communication channel has sufficiently low losses. This is because, in accordance with the fluctuation-dissipation theorem [17], the propagating photonic modes inside the communication channel are effectively decoupled from the ambient hot environment, thus preserving the quantum correlations therein. The fluctuation-dissipation theorem states that the variance of the voltage fluctuations $\langle V^2 \rangle$ due to the transmission line temperature $T$, within the single-side measurement bandwidth $B$, is given by

$$\langle V^2 \rangle = 2\hbar \int_{\omega_0 - B}^{\omega_0 + B} \coth\left(\frac{\hbar\omega}{2k_{\text{B}}T}\right) \varepsilon(\omega) d\omega, \tag{1}$$

where $\varepsilon(\omega)$ corresponds to the dissipation spectrum, determined by the Fourier-transformed voltage susceptibility of the system [18]. For the superconducting NbTi cables used in our experiment, the dissipation spectrum is determined by its ohmic resistance. Hence, we have $\varepsilon(\omega) \ll 1$ for frequencies well below the superconductor gap frequency, $\omega \ll \omega_\Delta$, where $\omega_\Delta/2\pi \simeq 370\,\text{GHz}$ for NbTi. Moreover, the characteristic thermal energy scale in our experiment is much smaller than the superconductor gap energy $\Delta(T)$, so we can neglect the surface resistance $R_{\text{s}} \propto \exp\left[-\Delta(T)/(k_{\text{B}}T)\right]$ of the superconducting cables [19, 20]. Considering Eq. 1, an extremely small $\varepsilon(\omega)$ strongly suppresses the contribution from the ambient thermal bath with temperature $T$, effectively decoupling the phononic environmental temperature and the photonic mode temperature. Although the fragile quantum states propagate through a hot thermal bath, interaction between the states and the bath are suppressed as long as the cable temperature remains well below the critical temperature of the superconductor. The thermal fluctuation spectrum in the microwave communication channel is instead limited by the temperatures of the strongly dissipative 30 dB attenuators in Alice.

The fluctuation-dissipation theorem can also be interpreted using the beam splitter model from quantum optics [7], where the coupled thermal photon number is given by $n_{\text{th}} = \varepsilon n_{\text{env}}$, with $\varepsilon$ the channel losses and $n_{\text{env}}$ the environmental

thermal occupation number. For vanishing losses $\varepsilon \to 0$, the coupled thermal noise $n_{\mathrm{th}}$ is strongly suppressed, despite a hot environment with $n_{\mathrm{env}} \gg 1$ surrounding the quantum channel. In our experimental setup, the superconducting NbTi cables have measured losses of around $1\,\mathrm{dB\,km}^{-1}$ at the carrier frequency of 5.35 GHz. Hence, only 0.02 thermal noise photons are admixed into the microwave signals as they travel through the 6 m long quantum link in a 4 K environment. Furthermore, such microwave signals can pass about 0.3 km of superconducting coaxial cable at 4 K before one average noise photon is injected into the signal mode.

## IV. MODEL FOR ANALOG QUANTUM TELEPORTATION OF COHERENT STATES

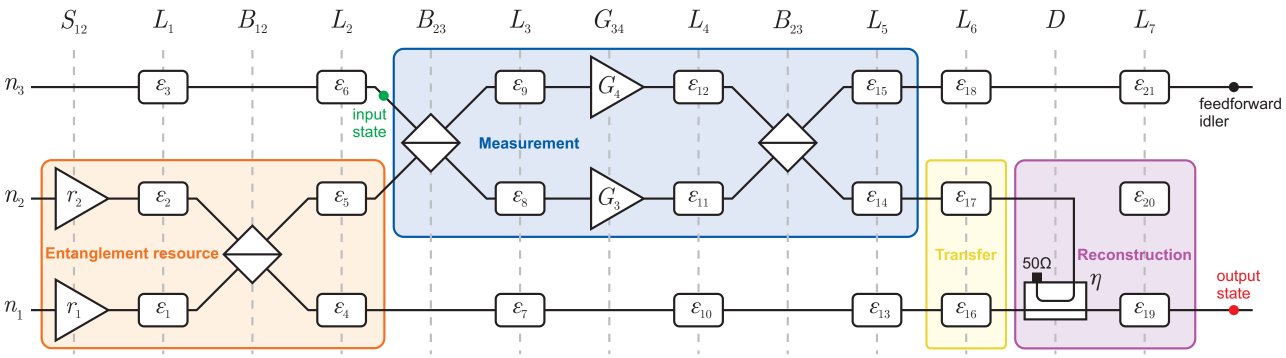


Supplementary Figure 3. Theory model for analog continuous-variable quantum teleportation.

In our implementation of the analog quantum teleportation protocol of coherent states, we utilize only Gaussian states and Gaussian operators. Hence, our quantum states can be described completely by their first and second order moments (mean and covariance, respectively). For the matrix representations, we use the basis $\{|p_1\rangle, |q_1\rangle, |p_2\rangle, |q_2\rangle, |p_3\rangle, |q_3\rangle\}$ where $|p_i\rangle, |q_i\rangle$ are the $p$-quadrature and $q$-quadrature components of mode $i$. We use $\mathbb{1}_2$ for the $2\times 2$ identity matrix, $\mathbb{0}_2$ for the $2\times 2$ zero matrix, and $\sigma_z$ for the Pauli-$z$ matrix. We use the vacuum variance definition of 1/4. Supplementary Figure 3 shows our full theory model, which includes all operators and path losses. The teleportation protocol is given by

$$\hat{T} = \hat{D}\hat{L}_7\hat{L}_6\hat{B}_{23}\hat{L}_5\hat{G}_{23}\hat{L}_4\hat{B}_{23}\hat{L}_3\hat{B}_{12}\hat{L}_2\hat{S}_{12}\hat{L}_1. \tag{2}$$

We write the squeezing operator as

$$\hat{S}_{12} = \hat{R}_{12}\hat{J}_{12}\hat{R}_{12}^{\dagger}, \tag{3}$$

with

$$\hat{J}_{12} = \begin{pmatrix} e^{-r_1} & 0 & 0 & 0 & 0 & 0 \\ 0 & e^{r_1} & 0 & 0 & 0 & 0 \\ 0 & 0 & e^{-r_2} & 0 & 0 & 0 \\ 0 & 0 & 0 & e^{r_2} & 0 & 0 \\ 0 & 0 & 0 & 0 & 1 & 0 \\ 0 & 0 & 0 & 0 & 0 & 1 \end{pmatrix}, \tag{4}$$

$$\hat{R}_{12} = \begin{pmatrix} \cos\gamma_1 & -\sin\gamma_1 & 0 & 0 & 0 & 0 \\ \sin\gamma_1 & \cos\gamma_1 & 0 & 0 & 0 & 0 \\ 0 & 0 & \cos\gamma_2 & -\sin\gamma_2 & 0 & 0 \\ 0 & 0 & \sin\gamma_2 & \cos\gamma_2 & 0 & 0 \\ 0 & 0 & 0 & 0 & 1 & 0 \\ 0 & 0 & 0 & 0 & 0 & 1 \end{pmatrix}. \tag{5}$$

We set the squeezing factors $r_1 = r_2 = r$ and the squeezing angles $\gamma_1 = 0$, $\gamma_2 = \pi/2$ for the TMS resource. We write the beam splitter operators

$$\hat{B}_{12} = \frac{1}{\sqrt{2}} \begin{pmatrix} \mathbb{1}_2 & \mathbb{1}_2 & \mathbb{0}_2 \\ -\mathbb{1}_2 & \mathbb{1}_2 & \mathbb{0}_2 \\ \mathbb{0}_2 & \mathbb{0}_2 & \sqrt{2}\mathbb{1}_2 \end{pmatrix}, \tag{6}$$

$$\hat{B}_{23} = \frac{1}{\sqrt{2}} \begin{pmatrix} \sqrt{2}\mathbb{1}_2 & \mathbb{0}_2 & \mathbb{0}_2 \\ \mathbb{0}_2 & \mathbb{1}_2 & \mathbb{1}_2 \\ \mathbb{0}_2 & -\mathbb{1}_2 & \mathbb{1}_2 \end{pmatrix}. \tag{7}$$

The measurement (phase-sensitive amplification) operator can be written as

$$\hat{G}_{23} = \hat{R}_{23}\hat{J}_{23}\hat{R}_{23}^{\dagger}, \tag{8}$$

with

$$\hat{J}_{23} = \begin{pmatrix} 1 & 0 & 0 & 0 & 0 & 0 \\ 0 & 1 & 0 & 0 & 0 & 0 \\ 0 & 0 & 1/\sqrt{G_3} & 0 & 0 & 0 \\ 0 & 0 & 0 & \sqrt{G_3} & 0 & 0 \\ 0 & 0 & 0 & 0 & 1/\sqrt{G_4} & 0 \\ 0 & 0 & 0 & 0 & 0 & \sqrt{G_4} \end{pmatrix}, \tag{9}$$

$$\hat{R}_{23} = \begin{pmatrix} 1 & 0 & 0 & 0 & 0 & 0 \\ 0 & 1 & 0 & 0 & 0 & 0 \\ 0 & 0 & \cos\gamma_3 & -\sin\gamma_3 & 0 & 0 \\ 0 & 0 & \sin\gamma_3 & \cos\gamma_3 & 0 & 0 \\ 0 & 0 & 0 & 0 & \cos\gamma_4 & -\sin\gamma_4 \\ 0 & 0 & 0 & 0 & \sin\gamma_4 & \cos\gamma_4 \end{pmatrix}. \tag{10}$$

We set the gains $G_3 = G_4 = G$ and the measurement angles $\gamma_3 = \gamma_1$, $\gamma_4 = \gamma_2$ for the Josephson interferometer. In order to genuinely implement analog quantum teleportation, the measurement gain must be large $G \gg 1$. We write the directional coupler operator

$$\hat{C} = \begin{pmatrix} \sqrt{1-\eta}\mathbb{1}_2 & \sqrt{\eta}\mathbb{1}_2 & \mathbb{0}_2 \\ -\sqrt{\eta}\mathbb{1}_2 & \sqrt{1-\eta}\mathbb{1}_2 & \mathbb{0}_2 \\ \mathbb{0}_2 & \mathbb{0}_2 & \mathbb{1}_2 \end{pmatrix}, \tag{11}$$

where $\eta$ is the coupling factor of the directional coupler. We express the loss operators for each segment $i$ of the experimental setup as

$$\hat{L}_i = \begin{pmatrix} \sqrt{1-\varepsilon_{3(i-1)+1}}\mathbb{1}_2 & \mathbb{0}_2 & \mathbb{0}_2 \\ \mathbb{0}_2 & \sqrt{1-\varepsilon_{3(i-1)+2}}\mathbb{1}_2 & \mathbb{0}_2 \\ \mathbb{0}_2 & \mathbb{0}_2 & \sqrt{1-\varepsilon_{3(i-1)+3}}\mathbb{1}_2 \end{pmatrix}. \tag{12}$$

We note that noise from the local thermal bath is coupled into the teleportation protocol via the local losses $\varepsilon_j$, which can be modeled as a beam splitter operation with transmissivity $\varepsilon_j$. The initial covariance matrix for Alice and Bob is given by

$$V_{\text{initial}} = \frac{1}{4} \begin{pmatrix} (1+2n_1)\mathbb{1}_2 & \mathbb{0}_2 & \mathbb{0}_2 \\ \mathbb{0}_2 & (1+2n_2)\mathbb{1}_2 & \mathbb{0}_2 \\ \mathbb{0}_2 & \mathbb{0}_2 & (1+2n_3)\mathbb{1}_2 \end{pmatrix}, \tag{13}$$

where $n_1$, $n_2$, $n_3$ is the input noise at each mode, respectively. At the start of the teleportation protocol, the first mode contains Bob's part of the TMS state, the second mode contains Alice's part of the TMS state, and the third mode contains Alice's input coherent state. The final covariance matrix is given by

$$V_{\text{final}} = \hat{T} V_{\text{initial}} \hat{T}^{\dagger} + N, \tag{14}$$

where the matrix $N$ represents the coupled noise due to losses in the protocol. We can simply extract the first mode of $V_{\text{final}}$ in order to obtain Bob's output state after the teleportation procedure. To perform a full simulation of our teleportation protocol, we use datasheet values to obtain exact numbers for the respective path losses $\varepsilon_j$. For each SMA connector, we estimate an additional 0.10 dB of losses due to impedance mismatch. These loss values are summarized in Table I.

Supplementary Table I. Microwave losses along specific segments in the experimental setup.

| Path | Microwave components | Total losses |
|---|---|---|
| $\varepsilon_1$ | 2 SMA connectors (0.20 dB) + circulator (0.15 dB) | 0.35 dB |
| $\varepsilon_2$ | 2 SMA connectors (0.20 dB) + circulator (0.15 dB) | 0.35 dB |
| $\varepsilon_3$ | no components | 0.00 dB |
| $\varepsilon_4$ | 1 SMA connector (0.10 dB) + hybrid ring (0.20 dB) | 0.30 dB |
| $\varepsilon_5$ | 2 SMA connectors (0.20 dB) + hybrid ring (0.20 dB) + switch (0.20 dB) | 0.60 dB |
| $\varepsilon_6$ | no components | 0.00 dB |
| $\varepsilon_7$ | no components | 0.00 dB |
| $\varepsilon_8$ | 1 SMA connector (0.10 dB) + hybrid ring (0.20 dB) + circulator (0.15 dB) | 0.45 dB |
| $\varepsilon_9$ | 1 SMA connector (0.10 dB) + hybrid ring (0.20 dB) + circulator (0.15 dB) | 0.45 dB |
| $\varepsilon_{10}$ | no components | 0.00 dB |
| $\varepsilon_{11}$ | 2 SMA connectors (0.20 dB) + circulator (0.15 dB) + switch (0.20 dB) | 0.55 dB |
| $\varepsilon_{12}$ | 2 SMA connectors (0.20 dB) + circulator (0.15 dB) + switch (0.20 dB) | 0.55 dB |
| $\varepsilon_{13}$ | no components | 0.00 dB |
| $\varepsilon_{14}$ | 1 SMA connector (0.10 dB) + hybrid ring (0.20 dB) | 0.30 dB |
| $\varepsilon_{15}$ | 1 SMA connector (0.10 dB) + hybrid ring (0.20 dB) | 0.30 dB |
| $\varepsilon_{16}$ | 6 m transmission superconducting cable (1 dB km$^{-1}$) | 0.006 dB |
| $\varepsilon_{17}$ | 6 m transmission superconducting cable (1 dB km$^{-1}$) | 0.006 dB |
| $\varepsilon_{18}$ | no components | 0.00 dB |
| $\varepsilon_{19}$ | 1 SMA connector (0.10 dB) + directional coupler (0.20 dB) | 0.30 dB |
| $\varepsilon_{20}$ | 1 SMA connector (0.10 dB) + directional coupler (0.20 dB) | 0.30 dB |
| $\varepsilon_{21}$ | no components | 0.00 dB |

The fidelity can by used to quantify the closeness of two quantum states. For single-mode Gaussian states, we use the Uhlmann fidelity [7, 14]

$$F(\alpha_1, V_1, \alpha_2, V_2) = \frac{1}{2}\frac{\exp\left(-\frac{1}{2}d^T(V_1+V_2)^{-1}d\right)}{\sqrt{\Lambda+\Delta}-\sqrt{\Delta}}, \tag{15}$$

$$\Lambda = \det(V_1+V_2), \tag{16}$$

$$\Delta = 16(\det V_1 - 1/16)(\det V_2 - 1/16), \tag{17}$$

$$d = \alpha_1 - \alpha_2, \tag{18}$$

where $\alpha_1$, $V_1$ and $\alpha_2$, $V_2$ are the displacement vectors and covariance matrices of state 1 and 2, respectively. In our analysis, we assume that the input state is a perfect coherent state with $V_{\text{input}} = \frac{1}{4}\hat{I}_2$. Thus, we get a simplified fidelity expression

$$F(d, v_{\text{out}}) = \frac{2}{1+4v_{\text{out}}}\exp\left(-\frac{2|d|^2}{1+4v_{\text{out}}}\right), \tag{19}$$

where $d$ is the displacement mismatch between the input and output states, and $v_{\text{out}}$ is the variance of the output state. We can then simulate our teleportation protocol by evolving an input coherent state using the teleportation operator in Eq. 2 and calculating the output state fidelity using Eq. 19. By fitting this theory model to our measured fidelity data, we get a simulated TMS resource squeezing parameter of $r = 0.778$ and measurement gain of $G = 21.47$ dB, which are very close to the calibrated operating parameters in our experiment $r = 0.790$ and $G = 21.76$ dB.

We can further simplify the theory model for our teleportation protocol by considering it as a noisy damping (or amplification) channel. The teleportation protocol essentially reconstructs Alice's input state as Bob's output state with a rescaling due to displacement mismatch and with added noise due to noisy devices, finite resource squeezing, and coupling to the environment via path losses. For infinitely large measurement gain, which is well-approximated by our experimental value $G \approx 21$ dB, we can write an analytical expression for the output state variance

$$v_{\text{out}} = \frac{1}{4}\left[\kappa + \eta\varepsilon W + (1+\kappa)\cosh 2r - 2\sqrt{\kappa}\sinh 2r\right], \tag{20}$$

where $\kappa = G\eta(1-\varepsilon)/4$ is the rescaling dependent on the gain $G$, directional coupling $\eta$, and total losses $\varepsilon$, and $W = 2n+1$ is the coupled noise from the ambient thermal photon number $n$. Thus, the teleported state fidelity can be written as

$$F(r,k,n) = \frac{2}{\zeta+\kappa+1}\exp\left[-2\frac{(\sqrt{\kappa}-1)^2}{\zeta+\kappa+1}|\alpha|^2\right], \tag{21}$$

$$\zeta = (1+\kappa)\cosh 2r - 2\sqrt{\kappa}\sinh 2r + n_{\mathrm{dev}} + n_{\mathrm{th}}, \tag{22}$$

where $\alpha$ is the input coherent state amplitude, $\kappa$ the effective gain, and $\zeta$ the effective added noise, $r$ the resource squeezing parameter, $n_{\mathrm{dev}}$ the added device noise, and $n_{\mathrm{th}}$ the coupled thermal noise. This expression takes into account the aggregate rescaling through $\kappa$ and the aggregate added noise through $\zeta$. By fitting this simplified theory model to our measured fidelity data, we get an aggregate rescaling of $\kappa = 0.778$ (or effective losses of 1.09 dB) and aggregate added noise of $\zeta = 1.015$. If we take the fitted TMS resource squeezing of $r = 0.778$, this implies device and coupled noise of $n = 0.304$ photons, of which 0.055 photons can be accounted for by gain-dependent JPA noise and 0.215 photons can be accounted for by coupling to the ambient thermal environment. If we take the fitted measurement gain of $G = 21.47$ dB, this implies total path losses of $\varepsilon = 1.56$ dB, which is very close to the estimate of 1.6 dB from datasheet values.

## V. MODEL FOR HYBRID QUANTUM TELEPORTATION OF QUBIT STATES

We now consider the hybrid quantum teleportation of Fock states with a TMS resource. The derivations follow the procedures in Refs. [21, 22]. Teleportation of Fock states $|n\rangle$ is possible because the TMS resource state contains contributions from all possible photon numbers. In order to model the analog quantum teleportation protocol for non-Gaussian states, we utilize the Wigner function formalism. We start with the three-mode Wigner function

$$W(q_1,p_1,q_2,p_2,q_3,p_3) = W_{\mathrm{TMS}}(q_1,p_1,q_2,p_2)W_{\mathrm{in}}(q_3,p_3), \tag{23}$$

$$W_{\mathrm{TMS}}(q_+,p_+,q_-,p_-) = \frac{4}{\pi^2}\exp\left[-\frac{2(q_+^2+p_-^2)}{e^{2r}} - \frac{2(q_-^2+p_+^2)}{e^{-2r}}\right], \tag{24}$$

where $W_{\mathrm{TMS}}$ describes the shared TMS resource state and $W_{\mathrm{in}}$ describes Alice's input state. This Wigner function transforms over the analog teleportation protocol according to

$$T^{-1} = \begin{pmatrix} \mathbb{1}_2 & -\sqrt{\eta}\mathbb{1}_2 & \mathbb{0}_2 \\ \sqrt{\kappa}\sigma_z & \sinh\phi\sigma_z & -\cosh\phi\mathbb{1}_2 \\ \sqrt{\kappa}\mathbb{1}_2 & \cosh\phi\mathbb{1}_2 & -\sinh\phi\sigma_z \end{pmatrix}, \tag{25}$$

where $\phi = (\ln G)/2$. The Wigner function of Bob's output state after this teleportation protocol is given by

$$W_{\mathrm{out}}(q_1,p_1) = \int W(T^{-1}R)dq_2dp_2dq_3dp_3, \tag{26}$$

where $R = (q_1,p_1,q_2,p_2,q_3,p_3)^{\intercal}$. We now perform the substitution

$$\begin{pmatrix}\tilde{q}_2\\ \tilde{p}_2\\ \tilde{q}_3\\ \tilde{p}_3\end{pmatrix} = \begin{pmatrix} \sinh\phi & 0 & -\cosh\phi & 0 \\ 0 & -\sinh\phi & 0 & -\cosh\phi \\ \cosh\phi & 0 & -\sinh\phi & 0 \\ 0 & \cosh\phi & 0 & \sinh\phi \end{pmatrix}\begin{pmatrix}q_2\\ p_2\\ q_3\\ p_3\end{pmatrix}. \tag{27}$$

Then, the phase-space coordinates of the final state is given by

$$q_1' = q_1 + \tilde{q}_2\sqrt{\eta}\sinh\phi - \tilde{q}_3\sqrt{\eta}\cosh\phi \simeq q_1 + \sqrt{\kappa}(\tilde{q}_2 - \tilde{q}_3), \tag{28}$$

$$p_1' = p_1 - \tilde{p}_2\sqrt{\eta}\sinh\phi - \tilde{p}_3\sqrt{\eta}\cosh\phi \simeq p_1 - \sqrt{\kappa}(\tilde{p}_2 + \tilde{p}_3), \tag{29}$$

where the approximation is approached for large $G \gg 1$. We find the output Wigner function

$$W_{\text{out}}(q_1, p_1) = \int W(q_1 + \sqrt{\kappa}(\tilde{q}_2 - \tilde{q}_3), p_1 - \sqrt{\kappa}(\tilde{p}_2 + \tilde{p}_3), \tilde{q}_2, \tilde{p}_2, \tilde{q}_3, \tilde{p}_3) d\tilde{q}_2 d\tilde{p}_2 d\tilde{q}_3 d\tilde{p}_3, \tag{30}$$

which describes the analog quantum teleportation protocol in the Wigner function formalism. We can use this formalism to extend our analysis to non-Gaussian states, such as for the hybrid teleportation of Fock states and qubit states. We now insert Eq. 24 into the first two modes of Eq. 30 to rewrite the output state Wigner function as a convolution integral

$$W_{\text{out}}(q, p) = \frac{1}{\kappa} \left[W_{\text{in}} * G_{\xi}\right] \left(\frac{q}{\sqrt{\kappa}}, \frac{p}{\sqrt{\kappa}}\right), \tag{31}$$

$$G_{\tau}(q, p) = \frac{1}{2\pi\tau} \exp\left(-\frac{q^2 + p^2}{2\tau}\right), \tag{32}$$

where $\xi = \zeta/2\kappa$ is the normalized noise function. In this way, the teleportation protocol is represented as a single Gaussian channel characterized by $\kappa$ and $\xi$, which describes its phase-space rescaling and Gaussian convolution, respectively. Next, we write the density matrix formalism for qubit teleportation, using a superoperator $\hat{T}$ to connect Alice's input state $\hat{\rho}_{\text{in}}$ and Bob's output state $\hat{\rho}_{\text{out}}$ given by

$$\hat{\rho}_{\text{out}} = \hat{T}(\hat{\rho}_{\text{in}}) = \sum_{m,n} \langle m|\hat{\rho}_{\text{in}}|n\rangle \sum_{j,l} T_{mn\to jl} |j\rangle \langle l|, \tag{33}$$

where $T_{mn\to jl}$ describes the complex transition probability amplitudes that map the input density matrix elements $|m\rangle\langle n|$ to the output elements $|j\rangle\langle l|$. Applying the Weyl-Wigner transformation, we get

$$W_{\text{out}}(q, p) = \sum_{m,n} \sum_{j,l} \langle m|\hat{\rho}_{\text{in}}|n\rangle\, T_{mn\to jl} W^{|j\rangle\langle l|}(q, p). \tag{34}$$

From Eq. 31, we can also write

$$W_{\text{out}}(q, p) = \sum_{m,n} \langle m|\hat{\rho}_{\text{in}}|n\rangle \frac{1}{\kappa} \left[W^{|m\rangle\langle n|} * G_{\xi}\right] \left(\frac{q}{\sqrt{\kappa}}, \frac{p}{\sqrt{\kappa}}\right). \tag{35}$$

By matching the coefficients, we have

$$\sum_{j,l} T_{mn\to jl} W^{|j\rangle\langle l|}(q, p) = \frac{1}{\kappa} \left[W^{|m\rangle\langle n|} * G_{\xi}\right] \left(\frac{q}{\sqrt{\kappa}}, \frac{p}{\sqrt{\kappa}}\right), \tag{36}$$

from which we can determine the transition probability amplitudes

$$T_{mn\to jl} = 2\pi \iint dqdp\; W^{|j\rangle\langle l|}(q, p) \frac{1}{\kappa} \left[W^{|m\rangle\langle n|} * G_{\xi}\right] \left(\frac{q}{\sqrt{\kappa}}, \frac{p}{\sqrt{\kappa}}\right). \tag{37}$$

We now restrict our analysis to the teleportation of pure qubit states

$$|\psi\rangle = \cos\frac{\theta}{2}|0\rangle + e^{i\varphi} \sin\frac{\theta}{2}|1\rangle, \tag{38}$$

on the Bloch sphere, and consider all transitions into Fock states $|n\rangle$ with $n \geq 2$ as leakage. Then, Bob's output state can be written as

$$\hat{\rho}_{\text{out}} = \rho_{00} |0\rangle\langle 0| + \rho_{10} |1\rangle\langle 0| + \rho_{01} |0\rangle\langle 1| + \rho_{11} |1\rangle\langle 1|, \tag{39}$$

$$\rho_{jl} = T_{00\to jl} \cos^2\frac{\theta}{2} + T_{10\to jl} e^{i\varphi} \cos\frac{\theta}{2} \sin\frac{\theta}{2} + T_{01\to jl} e^{-i\varphi} \cos\frac{\theta}{2} \sin\frac{\theta}{2} + T_{11\to jl} \sin^2\frac{\theta}{2}. \tag{40}$$

From Eq. 37, we can explicitly calculate the transition probability amplitudes

$$T_{00\to 00} = \frac{2}{\zeta + \kappa + 1}, \tag{41}$$

$$T_{00\to11} = 2\frac{\zeta+\kappa-1}{(\zeta+\kappa+1)^2}, \tag{42}$$

$$T_{11\to00} = 2\frac{\zeta-\kappa+1}{(\zeta+\kappa+1)^2}, \tag{43}$$

$$T_{11\to11} = \frac{2}{(\zeta+\kappa+1)^3}[(\zeta-\kappa+1)(\zeta+\kappa-1)+4\kappa], \tag{44}$$

$$T_{01\to01} = T_{10\to10} = \frac{4\sqrt{k}}{(\zeta+\kappa+1)^2}, \tag{45}$$

$$T_{00\to01} = T_{00\to10} = T_{11\to01} = T_{11\to10} = T_{01\to10} = 0, \tag{46}$$

$$T_{01\to00} = T_{10\to00} = T_{01\to11} = T_{10\to11} = T_{10\to01} = 0. \tag{47}$$

The Uhlmann fidelity between Alice's input state and Bob's output state is given by

$$F = \langle\psi|\hat{\rho}_{\text{out}}|\psi\rangle = \rho_{00}\cos^2\frac{\theta}{2} + \rho_{10}e^{i\varphi}\cos\frac{\theta}{2}\sin\frac{\theta}{2} + \rho_{01}e^{-i\varphi}\cos\frac{\theta}{2}\sin\frac{\theta}{2} + \rho_{11}\sin^2\frac{\theta}{2}, \tag{48}$$

which can be expressed as

$$F(\theta,\kappa,\zeta) = f_1(\kappa,\zeta) + f_2(\kappa,\zeta)\cos\theta + f_3(\kappa,\zeta)\cos 2\theta, \tag{49}$$

$$f_1(\kappa,\zeta) = \frac{\kappa^{\frac{3}{2}} + \sqrt{\kappa}(\zeta+1) + 2\zeta(\zeta+1) + 2\kappa(\zeta+3)}{(\zeta+\kappa+1)^3}, \tag{50}$$

$$f_2(\kappa,\zeta) = 2\frac{\zeta(\kappa+1)+(\kappa-1)^2}{(\zeta+\kappa+1)^3}, \tag{51}$$

$$f_3(\kappa,\zeta) = -\sqrt{\kappa}\frac{\zeta+(\sqrt{\kappa}-1)^2}{(\zeta+\kappa+1)^3}. \tag{52}$$

In particular, we have the ground state $|0\rangle$ teleportation fidelity

$$F(0,\kappa,\zeta) = \frac{2}{\zeta+\kappa+1}, \tag{53}$$

which recovers the scenario of teleporting a coherent state with $\alpha = 0$, and the excited state $|1\rangle$ teleportation fidelity

$$F(\pi,\kappa,\zeta) = \frac{2\zeta^2 - 2\kappa^2 + 12\kappa - 2}{(\zeta+\kappa+1)^3}. \tag{54}$$

We assume the capability to teleport arbitrary pure qubit states, so the average fidelity is determined by an integration over the Bloch sphere surface

$$\bar{F}(\kappa,\zeta) = \frac{1}{4\pi}\int_0^{2\pi}\int_0^{\pi} F(\theta,\kappa,\zeta)\sin\theta\ d\theta d\varphi = f_1(\kappa,\zeta) - \frac{1}{3}f_3(\kappa,\zeta). \tag{55}$$

The average qubit teleportation fidelity is then given by

$$\bar{F}(\kappa,\zeta) = \frac{6\zeta+4\sqrt{\kappa}}{3(\zeta+\kappa+1)^2} + \frac{16\kappa}{3(\zeta+\kappa+1)^3}. \tag{56}$$

For the case of an ideal teleportation protocol, where $\kappa = 1$, $n_{\mathrm{dev}} = 0$, and $n_{\mathrm{th}} = 0$, we get the ground state $|0\rangle$ teleportation fidelity

$$F_{|0\rangle}(r) = \frac{1}{1+e^{-2r}} = \frac{1+\tanh r}{2}, \tag{57}$$

the excited state $|1\rangle$ teleportation fidelity

$$F_{|1\rangle}(r) = \frac{1+e^{-4r}}{(1+e^{-2r})^3} = \frac{1}{4}(1+\tanh r)(1+\tanh^2 r), \tag{58}$$

and the average teleportation fidelity

$$\bar{F}(r) = \frac{3+4e^{-2r}+3e^{-4r}}{3(1+e^{-2r})^3}. \tag{59}$$

Finally, we notice that when performing hybrid quantum teleportation, the reconstructed state fidelities are lower for qubit states than for coherent states with the same average photon number. We can explain this by the orthogonality of Fock states, where $\langle n=0|n=1\rangle = \langle n=1|n=2\rangle = 0$. Meanwhile, for coherent states, we have $\langle \alpha=0|\alpha=1\rangle = \langle \alpha=1|\alpha=\sqrt{2}\rangle = 0.368$. Thus, if we view the quantum teleportation protocol as a noisy damping (or amplification) channel, the output state fidelity would deteriorate more quickly with rescaling for a Fock state than for a coherent state. Furthermore, losses severely limit the hybrid teleportation fidelity of Fock states by constraining the optimal TMS squeezing level [23]. It is possible to mitigate this limitation by utilizing dual-rail encodings of photonic qubits [24] or by employing superconducting microwave components [25, 26].

---


[1] W. K. Yam, M. Renger, S. Gandorfer, F. Fesquet, M. Handschuh, K. E. Honasoge, F. Kronowetter, Y. Nojiri, M. Partanen, M. Pfeiffer, H. van der Vliet, A. J. Matthews, J. Govenius, R. N. Jabdaraghi, M. Prunnila, A. Marx, F. Deppe, R. Gross, and K. G. Fedorov, npj Quantum Inf. **11**, 87 (2025).

[2] M. Mariantoni, E. P. Menzel, F. Deppe, M. A. Araque Caballero, A. Baust, T. Niemczyk, E. Hoffmann, E. Solano, A. Marx, and R. Gross, Phys. Rev. Lett. **105**, 133601 (2010).

[3] S. Gandorfer, M. Renger, W. Yam, F. Fesquet, A. Marx, R. Gross, and K. Fedorov, Phys. Rev. Appl. **23**, 024064 (2025).

[4] K. E. Honasoge, M. Handschuh, W. K. Yam, S. Gandorfer, D. Bazulin, N. Bruckmoser, L. Koch, A. Marx, R. Gross, and K. G. Fedorov, Phys. Rev. B **111**, 214508 (2025).

[5] T. Yamamoto, K. Inomata, M. Watanabe, K. Matsuba, T. Miyazaki, W. D. Oliver, Y. Nakamura, and J. S. Tsai, Appl. Phys. Lett. **93**, 042510 (2008).

[6] L. Zhong, E. P. Menzel, R. D. Candia, P. Eder, M. Ihmig, A. Baust, M. Haeberlein, E. Hoffmann, K. Inomata, T. Yamamoto, Y. Nakamura, E. Solano, F. Deppe, A. Marx, and R. Gross, New J. Phys. **15**, 125013 (2013).

[7] C. Weedbrook, S. Pirandola, R. García-Patrón, N. J. Cerf, T. C. Ralph, J. H. Shapiro, and S. Lloyd, Rev. Mod. Phys. **84**, 621 (2012).

[8] E. P. Menzel, R. Di Candia, F. Deppe, P. Eder, L. Zhong, M. Ihmig, M. Haeberlein, A. Baust, E. Hoffmann, D. Ballester, K. Inomata, T. Yamamoto, Y. Nakamura, E. Solano, A. Marx, and R. Gross, Phys. Rev. Lett. **109**, 250502 (2012).

[9] T. Yamashima, T. Kashiwazaki, T. Suzuki, R. Nehra, T. Nakamura, A. Inoue, T. Umeki, K. Takase, W. Asavanant, M. Endo, and A. Furusawa, Opt. Express **33**, 5769 (2025).

[10] R. Di Candia, K. G. Fedorov, L. Zhong, S. Felicetti, E. P. Menzel, M. Sanz, F. Deppe, A. Marx, R. Gross, and E. Solano, EPJ Quantum Technol. **2**, 25 (2015).

[11] F. Kronowetter, F. Fesquet, M. Renger, K. Honasoge, Y. Nojiri, K. Inomata, Y. Nakamura, A. Marx, R. Gross, and K. Fedorov, Phys. Rev. Appl. **20**, 024049 (2023).

[12] M. Renger, S. Pogorzalek, Q. Chen, Y. Nojiri, K. Inomata, Y. Nakamura, M. Partanen, A. Marx, R. Gross, F. Deppe, and K. G. Fedorov, npj Quantum Inf. **7**, 160 (2021).

[13] K. G. Fedorov, L. Zhong, S. Pogorzalek, P. Eder, M. Fischer, J. Goetz, E. Xie, F. Wulschner, K. Inomata, T. Yamamoto, Y. Nakamura, R. Di Candia, U. Las Heras, M. Sanz, E. Solano, E. P. Menzel, F. Deppe, A. Marx, and R. Gross, Phys. Rev. Lett. **117**, 020502 (2016).

[14] H. Scutaru, J. Phys. A **31**, 3659 (1998).

[15] S. L. Braunstein, C. A. Fuchs, H. J. Kimble, and P. van Loock, Phys. Rev. A **64**, 022321 (2001).

[16] F. Grosshans and P. Grangier, Phys. Rev. A **64**, 010301 (2001).

[17] H. B. Callen and T. A. Welton, Phys. Rev. **83**, 34 (1951).

[18] R. Kubo, J. Phys. Soc. Jpn. **12**, 570 (1957).

[19] J. P. Turneaure and I. Weissman, J. Appl. Phys. **39**, 4417 (1968).

[20] J. Bardeen, L. N. Cooper, and J. R. Schrieffer, Phys. Rev. **108**, 1175 (1957).

[21] S. Takeda, T. Mizuta, M. Fuwa, H. Yonezawa, P. van Loock, and A. Furusawa, Phys. Rev. A **88**, 042327 (2013).

[22] M. Renger, *Inter-lab Quantum Microwave Teleportation*, Ph.D. thesis, Technical University of Munich (2023).
[23] S. H. Lie and H. Jeong, Photon. Res. **7**, A7 (2019).
[24] S. Takeda, T. Mizuta, M. Fuwa, P. van Loock, and A. Furusawa, Nature **500**, 315 (2013).
[25] B. Kannan, A. Almanakly, Y. Sung, A. Di Paolo, D. A. Rower, J. Braumüller, A. Melville, B. M. Niedzielski, A. Karamlou, K. Serniak, A. Vepsäläinen, M. E. Schwartz, J. L. Yoder, R. Winik, J. I.-J. Wang, T. P. Orlando, S. Gustavsson, J. A. Grover, and W. D. Oliver, Nat. Phys. **19**, 394 (2023).
[26] R. Navarathna, D. T. Le, A. R. Hamann, H. D. Nguyen, T. M. Stace, and A. Fedorov, Phys. Rev. Lett. **130**, 037001 (2023).
